# Supplementary material for: Large voltage tuning of Dzyaloshinskii-Moriya Interaction: a route towards dynamic control of skyrmion chirality
Source: arXiv:1804.09955 source file (2018-06-26)
Supplement: Supplementary file 1 [file DMI_V_-nanoletters-suppl-revisions.pdf]

# Large Voltage Tuning of Dzyaloshinskii-Moriya Interaction: a Route towards Dynamic Control of Skyrmion Chirality-Supporting Information

Titiksha Srivastava,[†] Marine Schott,[†] Roméo Juge,[†] Viola Křižáková,[‡] Mohamed Belmeguenai,[¶] Yves Roussigné,[¶] Anne Bernand-Mantel,[‡] Laurent Ranno,[‡] Stefania Pizzini,[‡] Salim-Mourad Chérif,[¶] Andrey Stashkevich,[¶] Stéphane Auffret,[†] Olivier Boulle,[†] Gilles Gaudin,[†] Mairbek Chshiev,[†] Claire Baraduc,[†] and Hélène Béa*,[†]

†*Univ. Grenoble Alpes, CEA, CNRS, Grenoble INP*, INAC-Spintec, 38000 Grenoble, France, * Institute of Engineering Univ. Grenoble Alpes*

‡*Univ. Grenoble Alpes, CNRS, Institut Néel, F-38042 Grenoble, France*

¶*Laboratoire des Sciences des Procédés et des Matériaux, Univ. Paris 13 Nord, 93430 Villetaneuse, France*

E-mail: helene.bea@cea.fr

## S1: Optimization of material parameters to get skyrmionic bubbles

On thermally oxidized Si wafer, an underlayer of Ta (3nm) was deposited followed by deposition of $Fe_{72}Co_8B_{20}$ (0.9nm) and then a wedge of Ta (0.5-1.04nm) followed by natural oxidation. A capping layer of 0.5nm of Al was then deposited. All the depositions were made by DC magnetron sputtering. The samples were then annealed at 225°C. Due to the

wedge of top Ta, an oxidation gradient is formed as a function of its thickness. This leads to a variation of magnetic parameters along this wedge. The optimum oxidation of Ta results in higher anisotropy, whereas a lower (underoxidation) or a higher (overoxidation) oxidation leads to lower anisotropy (more details to be found in an article in preparation). In this study, we have used the underoxidized zone, where the domain wall energy with low anisotropy is further reduced with the interfacial DMI as it is given by $\sigma_W = 4\sqrt{AK} - \pi \mid D \mid$. It facilitates thermal demagnetization leading to stripe or labyrinthine domains which transform into skyrmion bubbles on applying small out of plane magnetic field ($30\mu T$) as indicated in inset of figure 1a in the main text. We have measured a magnetically dead layer of 0.25nm for the 0.9nm nominal thickness of FeCoB. The FeCoB thickness used in our calculation of the interfacial effects and the saturation magnetization is thus 0.65nm.

## S2: Motion under current

In order to study the motion of bubbles under current, we have used UV lithography and etching to pattern Hall crosses on the Ta/FeCoB/TaOx trilayer. The size of the contact pad is $150\mu m$. A constant out-of-plane magnetic field of $30\mu T$ is applied to form the bubbles. A DC current of 0.11 mA (leading to a current density of $2 \times 10^8 A/m^2$ in the $150\mu m$ pad) is applied between the contact pads so that it flows in the Ta/FeCoB metallic bilayer (as shown in Fig.1 and in the video). The motion of the skyrmionic bubbles is against the electron flow. A velocity of $\approx 20\mu m/s$ is obtained which is similar to the study by Jiang et al.[1] Their uniform and unidirectional motion indicates their non trivial topology and hence their skyrmionic nature.

## S3: Time scale effects and reversibility of measurements

We have observed with p-MOKE measurements that the equilibrium width of stripes evolve with the duration of voltage application. In order to better know the time constants of the

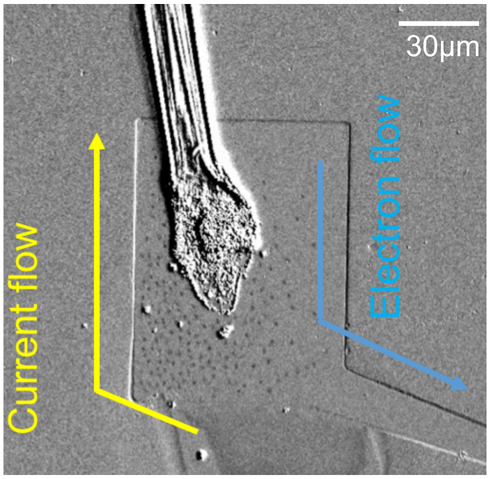


Figure 1: Polar Kerr image of skyrmionic bubbles under applied current (the wire of only one of the electrical pads is visible in the image). The arrows indicate the direction of current flow and electron flow. The skyrmion bubbles move uniformly against the electron flow.

physical mechanisms involved, we have performed p-MOKE with different time scales, from minutes to hours: we see in Fig 2 that a saturation is reached for 1h time scale.

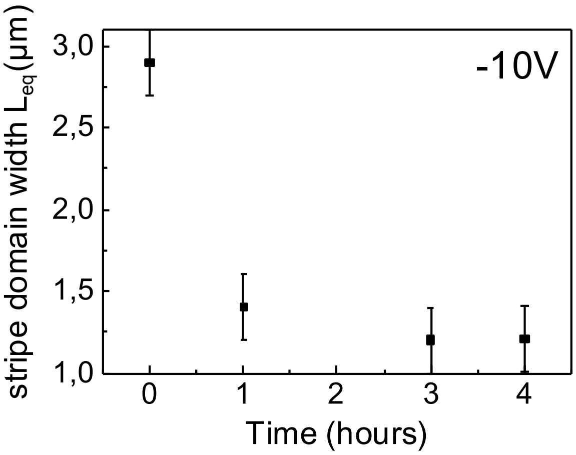


Figure 2: Evolution of $L_{eq}$ with applied voltage duration, as measured by p-MOKE microscopy.

As explained in the main text, in order to be in the same condition as the long BLS measurements we have performed long time p-MOKE measurements (4h). It thus corresponds to the saturation region. We have also measured over shorter time scales (few minutes, when the stripes have reached their equilibrium), as the short time scales may also be interesting from the point of view of applications. These different time scales are used to differentiate

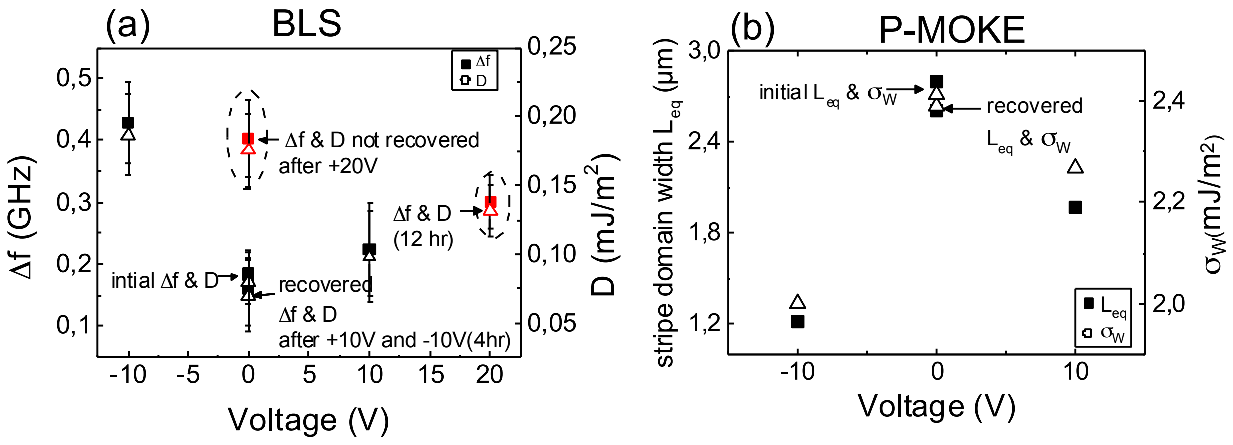


Figure 3: (a) Variation of frequency difference $\Delta f$ measured by BLS and deduced interfacial DMI as a function of applied voltage. The recovery of $\Delta f$ and hence the interfacial DMI at 0V after the measurements at -10V and 10V indicates the reversibility of the voltage effect. (b) Measured variation of stripe domain width p-MOKE and deduced domain wall energy as a function of applied voltage. The recovery of the values at 0V after long time scale measurements at -10V and 10V further confirms the reversibility of the voltage effect.

between charge effect, which would be present at both short and long time scales and ion migration or charge trapping which would occur only for longer time scale. These two types of measurements are presented in the main paper.

In order to check the reversibility of the voltage effect on magnetic parameters, the BLS measurements were repeated at 0V after the measurements under gate voltage. As indicated in Fig. 3a, the values of the frequency shift $\Delta f$ measured by BLS are recovered at 0V after long duration (4 hours) measurements at -10V and 10V indicating that there was no irreversible effect and also no damage to the electrodes during the measurements under voltage. The measurement at 0V was also performed with the in-plane magnetic field reversed to ensure the liability of the measurements: the opposite frequency difference was obtained, as expected.

Similarly, for the p-MOKE measurements, we have checked the equilibrium width of stripes under voltage for long application times (up to 4h). Up to + 10 or -10V for 4h, no irreversibility was observed. However on the application of higher voltage for durations longer than 10 hours, the changes became irreversible.

## S4: Evolution of $\Delta f$ with $k_{SW}$

We show here that the frequency difference varies linearly with the spin wavevector $k_{SW}$ (see fig. 4), which is expected for $\Delta f$: $\Delta f = \frac{2\gamma}{\pi M_s} k_{SW} D$.[2,3]

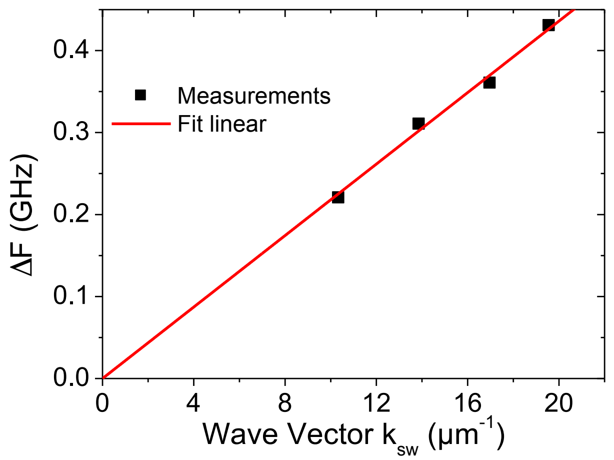


Figure 4: $\Delta f$ measured as a function of spin wave vector $k_{SW}$

In order to avoid electrode degradation, we have thus performed the BLS measurements under voltage at a fixed $k_{SW} = 20.45 \mu m^{-1}$, allowing shorter duration of the measurement.

## S5: Evolution of $M_s$ and $H_K$ with gate voltage

With p-MOKE microscopy, we have measured the evolution of the saturation magnetization and anisotropy field under gate voltage. $M_s$ evolution has been measured by the amplitude of the Kerr signal change when the magnetization is reversed, as represented by the arrow in the inset of Fig 5a. As only voltage changes, the Kerr signal is proportional to $M_s$ (other optical parameters are constants during these measurements performed in the same conditions). Its variation under voltage is presented in Fig 5a.

For the $H_k$ measurements, we have applied an in-plane field and measured Kerr signal. The fit of the obtained hard-axis curves leads to an estimation of the anisotropy field with voltage (see fig 5b). These measurements were made only on short time scales owing to the

imitations of experimental setup. 12% variation of $H_k$ is observed in the range of $\pm 10V$ for short time scales.

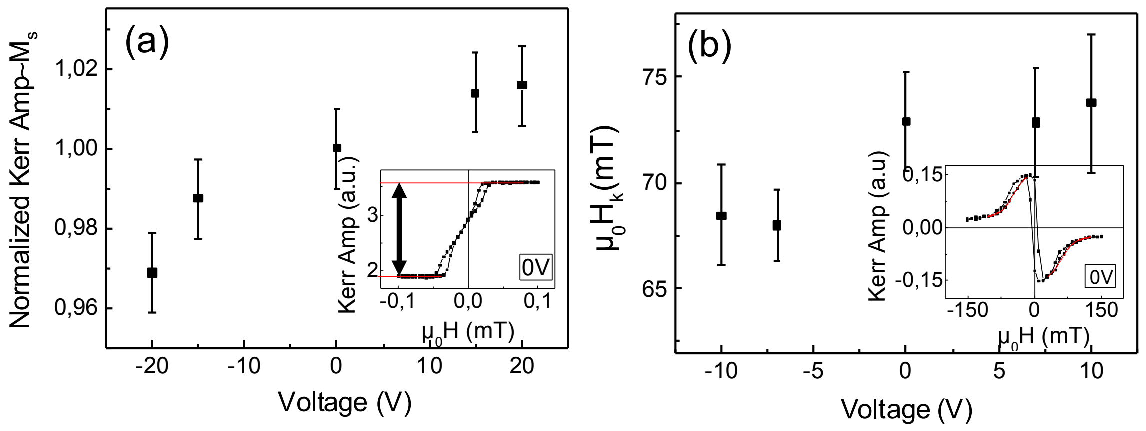


Figure 5: a) Variation under gate voltage of the amplitude of Kerr signal step (as represented by the arrow in inset) normalized by its value at 0V. It is proportional to saturation magnetization $M_s$. (Inset) Corresponding loop measured at 0V with out-of-plane field. (b) Variation under gate voltage of anisotropy field $H_k$. (Inset) Kerr signal loop for 0V with in-plane applied magnetic field. All these data are measured at short time scales.

## S6: Parameters measured and extracted on different time scales

In table 1, we have reported all experimental parameters used in the main text. They are given, when relevant, for the different applied voltages and at the two time scales, together with the measurement or extraction method.

## S7: Analytical model of isolated bubble and micromagnetic simulations

We have used the analytical model of isolated bubble developed in reference.[4] It takes into account the dipolar, exchange, anisotropy, Zeeman and DMI energies to calculate the energy of an isolated circular bubble depending on its diameter. The difference between this energy

Table 1: Summary of experimental parameters, with their measurement method, voltage and time scale

| Parameters | Voltage | 4h duration | Voltage | Few min duration | Method |
|---|---|---|---|---|---|
| $\Delta f$ (GHz) | 0V | 0.18 ±0.04 | | | BLS |
| | -10V | 0.43± 0.07 | | | |
| | 10V | 0.23± 0.07 | | | |
| $M_s(0V)$ (MA/m) | | | 1.05 | | SQUID |
| $M_s(V)/M_s(0V)$ | 0V | 1 | 0V | 1 | p-MOKE |
| | -10V | 0.94 ±0.01 | -20V | 0.96 ±0.01 | |
| | +10V | 0.94 ±0.01 | +20V | 1.02 ±0.01 | |
| $\mu_0 H_k(0V)$ (mT) | | | 73.0 | | SQUID |
| $\mu_0 H_k(V)/\mu_0 H_k(0V)$ | | | 0V | 1 | p-MOKE |
| | | | -10V | 0.95 ±0.05 | |
| | | | +10V | 1.06 ±0.05 | |
| $\sigma_W$ (mJ/m$^2$) | 0V | 2.37±0.3 | 0V | 2.21±0.2 | p-MOKE |
| | -10V | 1.84 ±0.3 | -20V | 1.84 ±0.2 | |
| | +10V | 2.21 ±0.3 | +20V | 2.41 ±0.2 | |
| $D$ (mJ/m$^2$) | 0V | 0.08±0.016 | 0V | 0.12±0.02 | BLS, p-MOKE |
| | -10V | 0.18 ±0.035 | -20V | 0.185 ±0.02 | |
| | +10V | 0.13 ±0.035 | +20V | 0.08 ±0.02 | |

and the energy of the ferromagnetic state is plotted in fig 6 for 3 sets of parameters (continuous line corresponds to +80V, 0.5mT, as in the figure of the main text). They are based on the -20V case (short time scale), for which we have measured and extracted magnetic parameters, and on +80V, with the parameters extrapolated from voltage measurements in the -20 / +20V range. For the +80V case, we have plotted the energy for two magnetic fields, $\mu_0$H=0.3 and 0.5 mT. In all three cases a bubble is stable. In the +80V case, the bubble has a larger diameter when the field is smaller, as expected. We have also added the calculation for +88V, which corresponds to a larger DMI (in absolute value). For this case, we had to apply 1mT to stabilize a bubble around $1\mu m$ diameter.

For the micromagnetic simulations, we have used the Mumax3 code,[5] which integrates numerically the Landau-Lifshitz-Gilbert equation. The Gilbert damping is set to $\alpha$=1 to decrease the relaxation time and temperature is 0K for simplicity. The geometry considered is a 6-$\mu$m-diameter disk with 5 nm x 5 nm cells. Initially, the disk is uniformly magnetized

($m_z > 0$) and a 2-$\mu$m-diameter bubble with opposite magnetization ($m_z < 0$) is generated in its center. The simulation relaxes the magnetic configuration to its lowest energy.

Using the experimental parameters, the evolution with voltage for the saturation magnetization $M_s$, the uniaxial anisotropy constant $K_u = K_s/t$ and DMI energy $D$ have been fitted in the -20/+20V range: : $M_s(V) = \eta_{M_s}V + M_s(0V)$ with $\eta_{M_s}$ = 1.575 $\times 10^3$ A/V/m and $M_s(0V)$ = 1.02 $\times 10^6$ A/m ; $K_u(V) = \eta_K V + K_u(0V)$ with $\eta_K$ = 2.1 $\times 10^3$ J.m$^{-3}V^{-1}$ and $K_u(0V) = 6.58 \times 10^5$ J.m$^{-3}$ and $D(V) = \eta_D V + D_0$ with $\eta_D$ = -0.0031 mJ.m$^{-2}V^{-1}$ and $D_0$ = 0.11 mJ.m$^{-2}$.

The exact parameters used in the model and the simulations are given in table 2. Starting from experimental parameters and fits, they have been slightly adjusted within the experimental error bars to lead to a stabilization of bubbles.

As shown in the main text, for -20V case, a bubble with outward pointing spins is obtained. In the +80V case, for a field of $\mu_0 H$=0.3mT, the micromagnetic simulations showed that the stabilized structures was not an isolated bubble but stripes. By increasing a bit the magnetic field (to 0.5mT) a single bubble could be stabilized again with spins in the domain wall pointing inward (as shown in the main paper). Consistently with these results, the analytical model showed an increased diameter of the bubble for 0.3 mT as compared to 0.5mT. However, the analytical model does not allow a non circular shape and such increased diameter could be in reality non isotropic and lead to stripe structure as obtained with the simulation.

We note here that the DMI value for the +80V is $-0.13 mJ/m^2$ and has not exactly the same absolue value as the -20V case ($+0.18 mJ/m^2$). The obtained Dzyaloshinskii wall for +80V case, as shown in the main text, is attributed to a value lower than the critical DMI.[6] We thus have tried simulations with increased DMI (in absolute value) $D = -0.16 mJ/m^2$, which corresponds to +88V applied voltage. In that case the domain wall energy becomes negative. However, with applied magnetic field, a bubble is stabilized, as shown in Fig. 6b. Here the obtained wall is purely Néel, which is consistent with the increased absolute value

of DMI.

We note here that the magnetic field is higher in our analytical calculation and micromagnetic simulation (0.3 to 1mT as compared to 30$\mu$T for experiments). This difference could be ascribed to the fact that in the model and the simulation we could not take into account the effect of other bubbles.

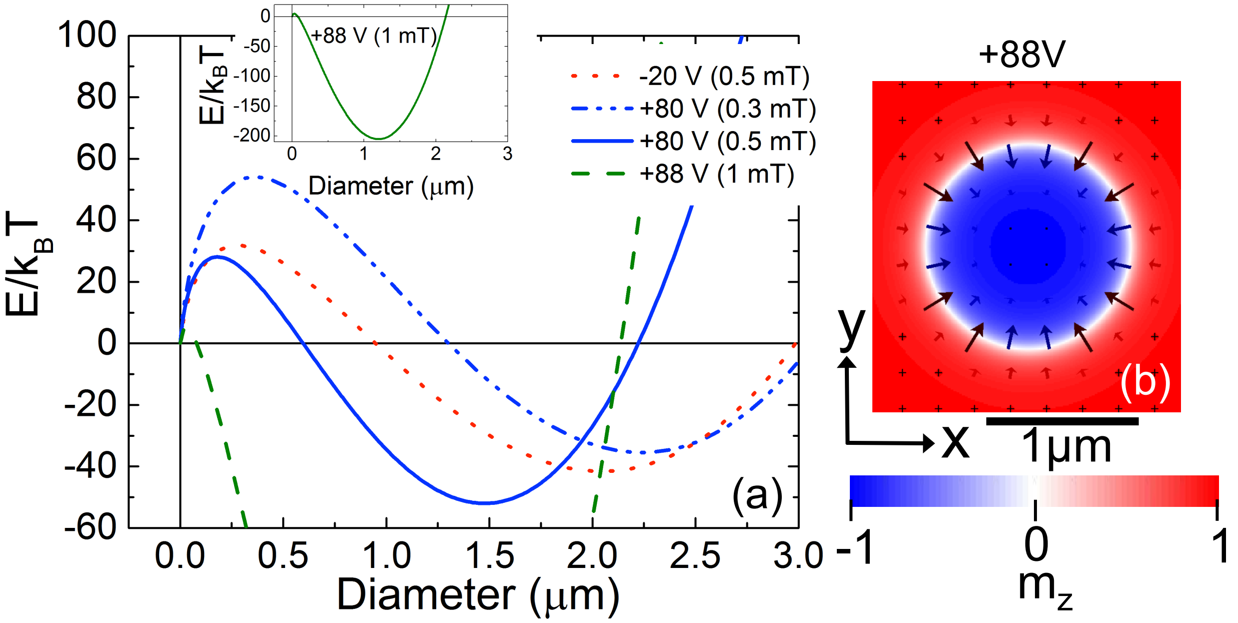


Figure 6: (a) Analytical model: variation of the energy difference between the bubble state and the saturated state as a function of the bubble diameter. The magnetic parameters are close to the ones measured previously for the -20V (short time) and extrapolated from the voltage variation of these parameters for the +80V and +88V. This latter voltages would correspond to negative DMI. In all cases, a stable bubble is obtained. For the +88V we had to apply a larger magnetic field to stabilize a bubble with similar size. In inset is represented the full curve for the +88V. (b) Micromagnetic simulations : distribution of magnetization of skyrmionic bubbles obtained in a 6 $\mu$m dot, under 1mT field, with parameters corresponding to the ones of the analytical model for +88V. Néel domain walls are obtained in that case.

First, the analytical model corresponds to a single isolated bubble. The calculation with 30$\mu$T lead to very large single bubble (20$\mu$m diameter). Such increase of diameter is not likely to occur in reality, but rather a distortion of the bubble or its separation in many bubbles is more plausible. A lower energy state is thus possible with several bubbles with smaller diameter.

Table 2: Parameters used for analytical model and for micromagnetic simulations

| $M_s$ (MA/m) | $K_s$ (mJ/m$^2$) | $D_s$ (pJ/m) | $A$ (pJ/m) | $t$ (nm) | $\mu_0$H (mT) | voltage (V) |
|---|---|---|---|---|---|---|
| Analytical model | | | | | | |
| 0.987 | 0.436 | +120.25 | 12 | 0.675 | 0.3 | -20 |
| 1.1447 | 0.575 | -91.2 | 12 | 0.675 | 0.3 | +80 |
| 1.1447 | 0.575 | -91.2 | 12 | 0.675 | 0.5 | +80 |
| 1.159 | 0.592 | -110 | 12 | 0.675 | 1 | +88 |
| Micromagnetic simulations | | | | | | |
| 0.987 | 0.418 | +120.5 | 12 | 0.68 | 0.3 | -20 |
| 1.1445 | 0.561 | -91 | 12 | 0.68 | 0.3 | +80 |
| 1.1445 | 0.561 | -91 | 12 | 0.68 | 0.5 | +80 |
| 1.157 | 0.572 | -108 | 12 | 0.68 | 1 | +88 |

Second, the micromagnetic simulations are done within a 6 $\mu$m dot in order to have reasonable calculation time. In that case, due to the edge effect, the presence of other bubbles will be less likely than in a infinite thin film. In the presence of other bubbles in the film, their repulsion interaction would result in a reduced size for a given magnetic field. Similarly to the analytical model, we thus had to increase the magnetic field in the simulation to obtain a micron-sized single bubble.

# References


(1) Jiang, W.; Upadhyaya, P.; Zhang, W.; Yu, G.; Jungfleisch, M.B.; Fradin, F.Y.; Pearson, J.E.; Tserkovnyak, Y.; Wang, K.L.; Heinonen, O.; te Velthuis, S.G.E.; Hoffmann, A. Blowing Magnetic Skyrmion Bubbles, *Science* **2015**, *349*, 283, DOI: 10.1126/science.aaa1442

(2) Belmeguenai M.; Gabor M. S.; Roussigné Y.; Stashkevich A.; Chérif S. M.; Zighem F.; Tiusan C. Brillouin light scattering investigation of the thickness dependence of Dzyaloshinskii-Moriya interaction in $Co_{0.5}Fe_{0.5}$ ultrathin films, *Phys. Rev. B* **2016**, *93*, 174407, DOI:10.1103/PhysRevB.93.174407

(3) Belmeguenai M.; Adam, J-P.; Roussigné Y.; Eimer S.; Devolder T.; Kim J-V.; Cherif

S-M.; Stashkevich A.; Thiaville A. Interfacial Dzyaloshinskii-Moriya interaction in perpendicularly magnetized Pt/Co/$AlO_x$ ultrathin films measured by Brillouin Light spectroscopy, *Phys. Rev. B* **2015**, *91*, 180405(R), DOI:10.1103/PhysRevB.91.180405

(4) Schott M.; Bernand-Mantel, A.; Ranno, L.; Pizzini, S.; Vogel, J.; Béa, H.; Baraduc, C.; Auffret, S.; Gaudin, G.; Givord, D. The Skyrmion Switch: Turning Magnetic Skyrmion Bubbles on and off with an Electric Field, *NanoLett.*, **2017**, *17*, 3006, DOI: 10.1021/acs.nanolett.7b00328

(5) Vansteenkiste A.; Leliaert J.; Dvornik M.; Helsen M.; Garcia-Sanchez F.; Van Waeyenberge B. The design and verification of MuMax3, *AIP Advances* **2014**, *4*, 107133, DOI:10.1063/1.4899186

(6) Thiaville, A.; Rohart, S.; Jué, E. ; Cros, V.; Fert, A. Dynamics of Dzyaloshinskii domain walls in ultrathin magnetic films, *Europhys. Lett.* **2012**, *100*, 57002, DOI:10.1209/0295-5075/100/57002
